# Supplementary material for: Active World Model Learning with Progress Curiosity
Source: arXiv:2007.07853 source file (2020-07-15)
Supplement: Supplementary file 2 [file wm_architecture.tex]

\section{World model architecture ablation and disentanglement}
\label{sec:app:wm_architecture}

To evaluate the importance of disentanglement in world model architecture, independently of controller choice, we produce datasets for offline training for each task (excluding peekaboo, since the behavior is dependent on the observer's choices, no policy-independent offline training dataset can be constructed). We then train the world model to convergence. We compare the loss of our disentangled world model to an \textit{entangled} LSTM architecture that instead takes as input and predicts all external agents together. As seen in Figure~\ref{fig:offline_asymptotic_performance}, the disentangled architecture significantly outperforms the entangled ablation.

\begin{wrapfigure}{R}{0.5\textwidth}
\vspace{-10pt}
\begin{center}
    \includegraphics[width=.5    \textwidth]{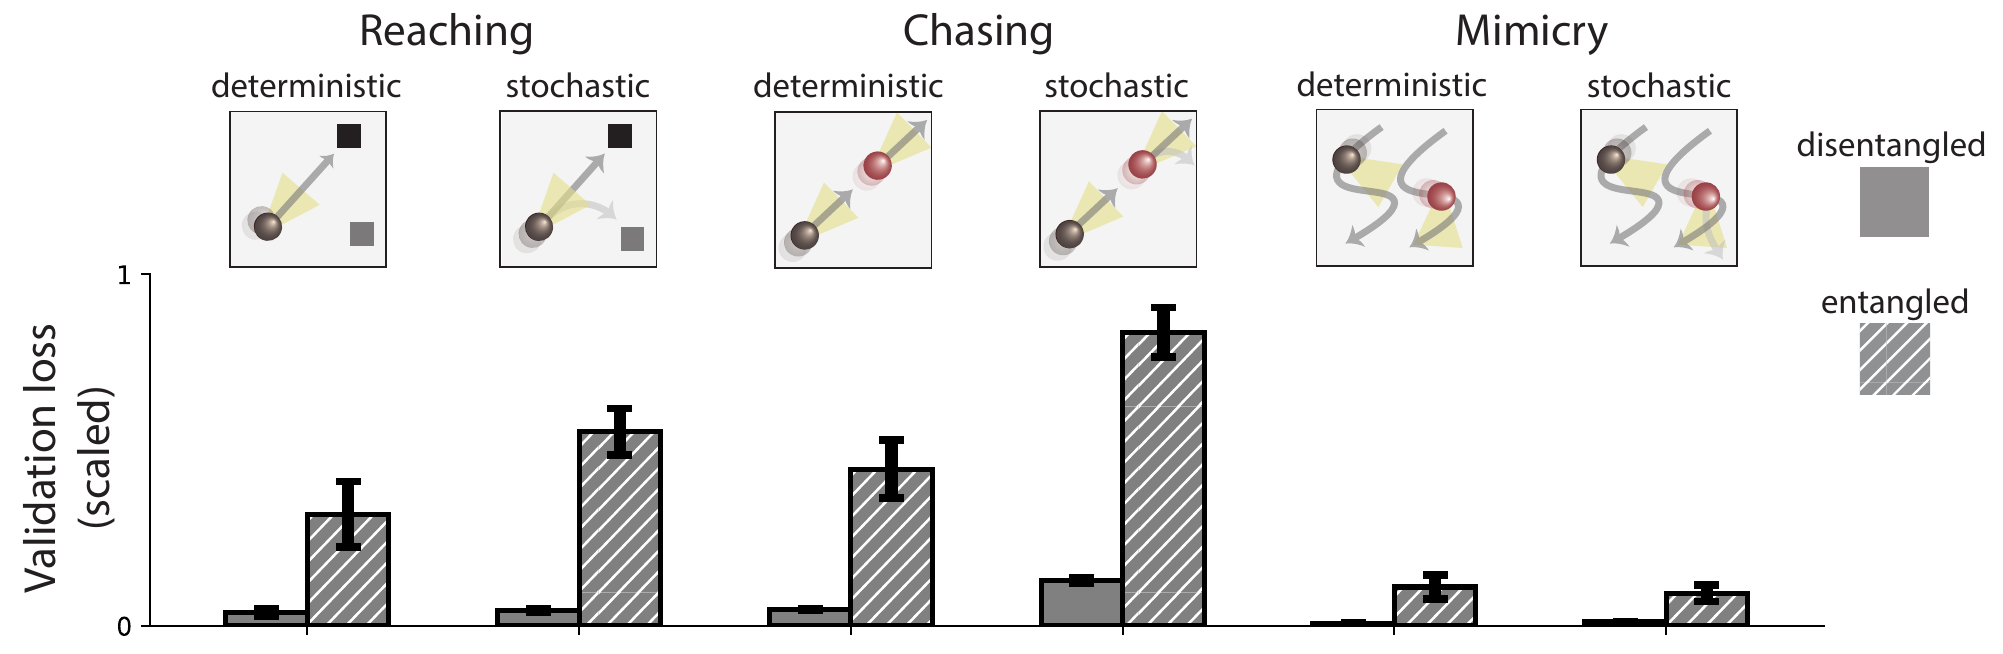}
\end{center}
\vspace{-10pt}
    \caption{\textbf{Asymptotic Model Performance} Final performance of the disentangled world model and entangled ablations.}
    \label{fig:offline_asymptotic_performance}
\vspace{-10pt}
\end{wrapfigure}

Intuitively, the disentangled architecture performs better because it ignores spurious correlations between causally-unrelated events in the agent's data stream.
Formalizing this intuition and explaining why this is particularly salient in our current environment, in contrast to some other situations \citep{locatello2018challenging}, is an important future direction.
Interestingly, the disentangled architecture shares a key feature with the concept known as Theory of Mind, which involves the ability to predict the behaviors of other agents as a function of inferred mental states, such as beliefs, desires, and goals \cite{astington1990developing, premack1978does, wellman1992child}.
A core, though often unstated, assumption behind Theory of Mind is the agent-centric allocation of computational resources.
Our disentangled model builds this in as a key feature, suggesting that at least one possible function of Theory of Mind may be to enable statistical disentangling.
This certainly requires considerable follow-up work to substantiate.
