# Supplementary material for: Active World Model Learning with Progress Curiosity
Source: arXiv:2007.07853 source file (2020-07-15)
Supplement: Supplementary file 5 [file GAL_AL_connection.tex]

\section{Connections between General Active Learning and Conventional Active Learning}
\label{sec:app:gal_cal_connection}

\textbf{Query Synthesis Active Learning} is obtained by taking $\S = \Y, \A = \X, P(\cdot | \cdot, \rva=\rvx) = \omega(\rvx)$ and $c(\bar{\rvs} = (\rvs, H, \theta), \rva, \bar{\rvs}' = (\rvs', H', \theta')) = \LL_{val}(\theta) - \LL_{val}(\theta')$. In words, the agent proposes a synthetic data query $\rva$ and the oracle $P$ provides a label $\rvs'$. The agent's objective is to reduce validation loss with a minimal number of data queries. Most active learning methods take a greedy approach to maximize the model loss reduction after a single data query which corresponds to setting $\beta = 0$. 

\textbf{Pool-based Active Learning} is the same as Query Synthesis Active Learning with the only difference being $\A = \mc{D}_{pool}$ where $\mc{D}_{pool}$ is the initial pool of unlabelled data. 

\textbf{Stream Active Learning} is obtained by choosing $\S = \X \times \Y, \A = \{0, 1\}, P(\cdot | \rvs=(\rvx, \rvy), \rva) = \omega(\rvx)~\text{if}~\rva = 1~\text{else}~\delta(\rvy_{dum})$, and $c(\bar{\rvs} = (\rvs, H, \theta), \rva, \bar{\rvs}' = (\rvs', H', \theta')) = \LL_{val}(\theta) - \LL_{val}(\theta')$, where $\delta$ is the Dirac-delta function and $\rvy_{dum}$ is a dummy label that denotes the case when no label is returned by the oracle.
