# Supplementary material for: Active World Model Learning with Progress Curiosity
Source: arXiv:2007.07853 source file (2020-07-15)
Supplement: Supplementary file 13 [file future.tex]

\section{Future Directions}
\label{sec:app:future}

Yet scalable intrinsic motivation is only one piece of curiosity, and we see at least two key related activities. The first concerns the agent's world model: what makes a good world model for environments with other agents? Initial results suggest an important architectural motif, and it remains to validate this and more broadly develop computational ``theory of mind''. The second concerns how humans navigate a social world: how does the model compare to human behavior? Can we model child development with models such as these? In what follows, we describe progress in answering these questions as well as important next steps.

\subsection{World models of other agents and theory of mind}

The world model architecture of Section~\ref{sec:methods:worldmodel} reflects choices made to guarantee acceptable prediction performance if given good enough data. In particular, a {\em Theory of Mind v0} motif, which allocates separate models for separate external agent behaviors, may be crucial.  To test this, we construct an ``ideal dataset'' and compare final performance of this {\em causal} world model against two ablations: a {\em joined} acausal ablation that takes all observations and predicts all agents jointly, and a {\em split} acausal ablation that handles each external agent (as opposed to behavior) separately.  As seen in Figure~\ref{fig:offline_asymptotic_performance}, across all experiments, the causal world model significantly outperforms the ablations. For details, see Appendix~\ref{sec:offline}.

The reason for this performance difference may be understood in terms of {\em disentanglement}, in which the model finds spurious dependence on ``nuisance factors'' --- some external agents are irrelevant to the behavior of others. It may be that poor disentanglement is more likely to occur and be detrimental to generalization performance when learning world models of partially observable environments via interactive learning. For a formalization of disentanglement and further discussion regarding the challenge in our setting, see Appendix~\ref{sec:app:causal}.

The choice of term {\em Theory of Mind v0} is deliberate because `theory of mind' is also used to refer to the more sophisticated ability to predict the behaviors of other agents as a function of inferred mental states, such as beliefs, desires, and goals \citep{astington1990developing, premack1978does, wellman1992child}. The above motif represents a proto-version of this in which an agent, upon detecting agents or other stimuli in its environment, infers a causal structure  and allocates modules of its world model that respect the structure. In future work, we will look to both (1) build a system that can infer this causal prior from data and (2) stress-test its utility in a suitable range of environments --- in particular, those with changing causal structure and greater interplay between causal structure and partial observability.

\subsection{Modeling human behavior}

% \begin{wrapfigure}{hR}{0.4\textwidth}
% \vspace{-20pt}
% \begin{center}
%     \includegraphics[width=0.4\textwidth]{figures/humans_v4.pdf}
% \end{center}
% \vspace{-20pt}
%     \caption{\textbf{Ongoing human subject model comparison} Human adults wear a mobile eye tracker while watching displays consisting of four sets of self-propelled, spherical robots travelling along a mat. Human and model fixation proportions are similar.}
%     \label{fig:human_subject_experiment}
% \vspace{-10pt}
% \end{wrapfigure}

\begin{figure}
    \centering
    \includegraphics[width=\textwidth]{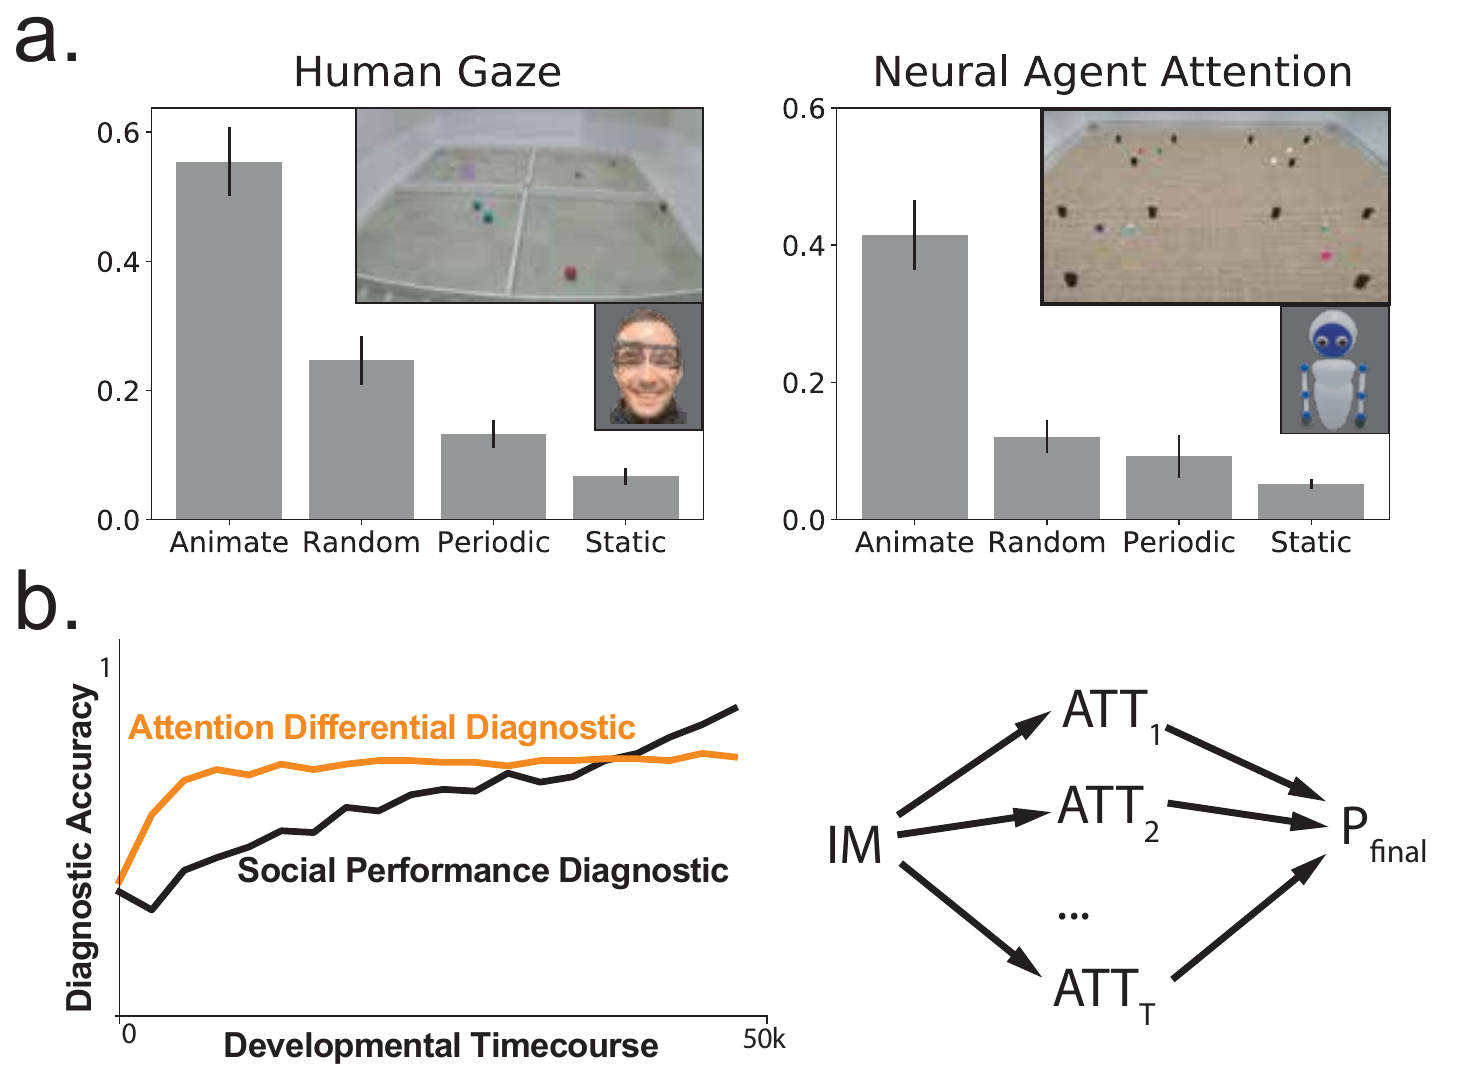}
    \vspace{-20pt}
    \caption{\textbf{Modeling human behavior}. (a-d) Human adults wear a mobile eye tracker while watching displays consisting of four sets of self-propelled, spherical robots travelling along a mat. Human and model fixation proportions are similar. (e) Accuracy of early performance and early attention predictors of final performance, as a function of $T$. (f) Factor analysis hypothesis: intrinsic motivation (IM) determines attention, which determines final performance.}
    \label{fig:human_modeling_combined}
    \vspace{-20pt}
\end{figure}

As a first step towards developing models of human behavior, we would like to quantify how humans explore a similar environment and make model comparison. In ongoing work, we are running human subject experiments in which we convey static, periodic, animate, and noise stimuli to humans via self-propelled, spherical robots moving along a mat, while measuring patterns of attention via a mobile eye tracker. So far, we find average fixation proportions favoring the animate stimuli. Furthermore, a $\gamma$-Progress network tasked to predict the virtual robot trajectories produces a similar aggregate attentional fixation pattern (Figure~\ref{fig:human_modeling_combined}a-d). A standard cognitive hypothesis is that the brain has a built-in module that specifically detects animacy from visual input \citep{leslie1989autism, leslie1994tomm}. Modeling results suggest that animate attention may instead arise from a more general curiosity-driven learning process.

% \begin{wrapfigure}{R}{0.4\textwidth}
% \vspace{0pt}
% \begin{center}
%     \includegraphics[width=.4 \textwidth]{figures/early_indicator_analysis_with_factor_analysis_v2.pdf}
% \end{center}
% \vspace{-10pt}
%     \caption{\textbf{Early indicator analysis}. (a) Accuracy of early performance and early attention predictors of final performance, as a function of $T$. (b) Factor analysis hypothesis: intrinsic motivation (IM) determines attention, which determines final performance.}
%     \label{fig:earlypredictor}
% \vspace{-10pt}
% \end{wrapfigure}

If we can model adult human behavior, can we model early childhood development? Can we model human developmental variability? If models can represent typical development, then it is possible that implementation variations (e.g. in intrinsic motivation signal) correspond to variability in development. Consider the following interpretation of the experiments of Section~\ref{sec:experiments} as a toy model of early childhood attention and learning. The ``population'' of agents have differently-implemented curiosity: differing intrinsic motivations represent underlying neural/genotype/phenotype correlates of early learning differences. Attention patterns represent objective behavioral measures of exploratory strategies (e.g. visual attention to eyes and mouths), and validation performance represents a more difficult to obtain measure of social acuity. An early behavioral measure that predicts outcomes later in life may provide both a valuable diagnostic criterion and a cue for possible interventions.

We test whether attention {\em early} in a run predicts {\em final} validation performance, and in particular whether, sufficiently early in a run, attention is a better predictor than early validation performance. We hence train two models:
\begin{enumerate}
    \item PERF$_{\leq T}$, which takes as input performance before time $T$, and stimulus type, and
    \item ATT$_{\leq T}$, which takes as input a summary of attention before time $T$, and stimulus type.
\end{enumerate}
As seen in Figure~\ref{fig:human_modeling_combined}e, ATT$_{\leq T}$ dominates until late (see Appendix~\ref{sec:app:attention_diagnostic} for details). Intuitively, as captured in the factor analysis diagram of Figure~\ref{fig:human_modeling_combined}f, we expect performance to be determined by attention throughout the run. Attention drives intrinsic motivation (see Appendix~\ref{sec:app:attention_determinants}, and if the intrinsic motivation can be inferred early, this predicts later attention and hence performance. This hence provides both an hypothesis for variation in human development, as well as a toy example of a behavioral trait that allows one to ``diagnose'' early.
